# Supplementary material for: MIMICause: Representation and automatic extraction of causal relation types from clinical notes
Source: arXiv:2110.07090 source file (2022-03-14)
Supplement: Supplementary file 1 [file appendix.tex]

% \section{Appendix}

% \setcounter{magicrownumbers}{0}
% \begin{center}
% \begin{longtable}{c c c c}
%     \caption{Sample sentences, guidelines and their annotations}
%     \label{tab:annotation_demo} \\
%     \toprule
%          S.No. & Sentence & Guideline & Annotation \\
%     \midrule
%     \endfirsthead
    
%     \multicolumn{4}{c}%
%     {{\tablename\ \thetable{} -- ... continued from previous page}} \\
%     \toprule
%          S.No. & Sentence & Guideline & Annotation \\
%     \midrule
%     \endhead
    
%          \multicolumn{4}{r}{{Continued on next page ...}} \\
%     \bottomrule
%     \endfoot
    
%     \bottomrule
%     \endlastfoot
    
%          \rownumber & \begin{minipage}{6cm} Odynophagia: Was presumed due to \textcolor{blue}{\textbf{\textless e2\textgreater mucositis\textless /e2\textgreater}} from recent \textcolor{red}{\textbf{\textless e1\textgreater chemotherapy\textless /e1\textgreater}}. \end{minipage} & \begin{minipage}{6cm} Single therapy ($e_1$) led to the effect ($e_2$) \end{minipage}  & Cause($e_1,e_2$) \\
%     \midrule
%          \rownumber & \begin{minipage}{6cm} \# \textcolor{red}{\textbf{\textless e1\textgreater Hypoglycemia\textless /e1\textgreater}}: Her presentation was related to aggressive increase in oral \textcolor{blue}{\textbf{\textless e2\textgreater hypoglycemics\textless /e2\textgreater}}, after her hypoglycemic medication dosages had been recently increased. \end{minipage} & \begin{minipage}{6cm} Increase of plural drugs as single entity ($e_2$) leading to $e_1$ \end{minipage} & Cause($e_2,e_1$) \\
%     \midrule
%          \rownumber & \begin{minipage}{6cm} While on the floor, you again had an abrupt change in your mental status where you were \textcolor{blue}{\textbf{\textless e2\textgreater hallucinating\textless /e2\textgreater}} and feeling very paranoid; it is thought that this was due to your high \textcolor{red}{\textbf{\textless e1\textgreater steroid\textless /e1\textgreater}} dose which has since been stopped. \end{minipage} & \begin{minipage}{6cm} High or low dosage of a single drug ($e_1$) led to hallucination ($e_2$) \end{minipage} & Cause($e_1,e_2$) \\
%     \midrule
%          \rownumber & \begin{minipage}{6cm} This was almost certainly due to an \textcolor{red}{\textbf{\textless e1\textgreater allergic reaction\textless /e1\textgreater}} to the medication lisinopril.Avoid this medication in the future and all other medications of this class, called ACE inhibitors or \textcolor{blue}{\textbf{\textless e2\textgreater angiotensin converting enzyme inhibitors\textless /e2\textgreater}}. \end{minipage} & \begin{minipage}{6cm} Phrase represents a single entity ($e_2$) which caused $e_1$ \end{minipage} & Cause($e_2,e_1$) \\
%     \midrule
%          \rownumber & \begin{minipage}{6cm} \# \textcolor{red}{\textbf{\textless e1\textgreater Normocytic Anemia\textless /e1\textgreater}} - Was 32.8 at OSH; after receiving fluids HCT has fallen further to 30.Baseline is 35 - 40.Not clinically bleeding.Perhaps due to \textcolor{blue}{\textbf{\textless e2\textgreater chemotherapy\textless /e2\textgreater}}. \end{minipage} & \begin{minipage}{6cm} Single therapy ($e_2$) led to $e_1$, expressed with uncertainty \end{minipage} & Cause($e_2,e_1$) \\
%     \midrule
%          \rownumber & \begin{minipage}{6cm} This was attributed to \textcolor{red}{\textbf{\textless e1\textgreater Vitamin K deficiency\textless /e1\textgreater}} secondary to \textcolor{blue}{\textbf{\textless e2\textgreater antibiotic\textless /e2\textgreater}} use, malnutrition and malabsorption from congested bowels related to decompensated CHF. \end{minipage} & \begin{minipage}{6cm} $e_2$ one of the contributiong factors leading to $e_1$ \end{minipage} & Enable($e_2,e_1$) \\
%     \midrule
%          \rownumber & \begin{minipage}{6cm} **], on recommendation from the pain service, patient's \textcolor{red}{\textbf{\textless e1\textgreater MS Contin\textless /e1\textgreater}} dose was increased to 160 mg TID from 130 mg TID, in addition to being ordered for PRN Dilaudid.Later that night, Pt fell while ambulating.He had a CT scan which was negative for acute intracranial pathologu. Morning after the fall, Pt was noted to be somnolent and \textcolor{blue}{\textbf{\textless e2\textgreater hypotensive\textless /e2\textgreater}}. \end{minipage} & \begin{minipage}{6cm} Increase in dosage of a drug ($e_1$) contributing in part leading to $e_2$ \end{minipage} & Enable($e_1,e_2$) \\
%     \midrule
%          \rownumber & \begin{minipage}{6cm} 4.\textcolor{blue}{\textbf{\textless e2\textgreater UTI\textless /e2\textgreater}} Urine culture from [**7-9**] grew $>100,000$ E coli, treated with \textcolor{red}{\textbf{\textless e1\textgreater ceftriaxone\textless /e1\textgreater}}. \end{minipage} & \begin{minipage}{6cm} Explicitly mentioned that state improved / disease ($e_2$) treated or controlled with a single drug ($e_1$) \end{minipage} & Prevent($e_1,e_2$) \\
%     \midrule
%          \rownumber &  \begin{minipage}{6cm} The patient was started on IV \textcolor{blue}{\textbf{\textless e2\textgreater ceftriaxone\textless /e2\textgreater}} which would cover both his UTI and \textcolor{red}{\textbf{\textless e1\textgreater balantitis\textless /e1\textgreater}}. \end{minipage} & \begin{minipage}{6cm} Single drug ($e_2$) expected to cure $e_1$ even though outcome not explicitly stated \end{minipage} & Prevent($e_2,e_1$) \\
%     \midrule
%          \rownumber & \begin{minipage}{6cm} During this period of suspected sepsis your \textcolor{red}{\textbf{\textless e1\textgreater seizure\textless /e1\textgreater}} frequency was noted to be higher than baseline.  We have adjusted your \textcolor{blue}{\textbf{\textless e2\textgreater anti-seizure medications\textless /e2\textgreater}} during the hospitalization. \end{minipage} & \begin{minipage}{6cm} Plural drugs ($e_2$) as one phrase for the treatment of $e_1$ \end{minipage} & Prevent($e_2,e_1$) \\
%     \midrule
%          \rownumber & \begin{minipage}{6cm} with chest and \textcolor{red}{\textbf{\textless e1\textgreater abdominal pain\textless /e1\textgreater}} and odynophagia who was found to have circumferential mural thrombus in the supra-renal aorta on cross sectional imaging.At that time the aortic pathology was though to be chronic.Ultimately, her pain resolved with the initiation of a \textcolor{blue}{\textbf{\textless e2\textgreater PPI\textless /e2\textgreater}} and GI cocktail, and was discharged home after a 3 day hospital stay. \end{minipage} & \begin{minipage}{6cm} Explicitly mentioned that pain ($e_1$) resolved with $e_2$ in coordination with another drug. \end{minipage} & Hinder($e_2,e_1$) \\
%     \midrule
%          \rownumber & \begin{minipage}{6cm} Cardiomyopathy and renal failure on current admission were felt to be manifestation of underlying \textcolor{blue}{\textbf{\textless e2\textgreater lupus\textless /e2\textgreater}}. Rheumatology was consulted and recommended aggressive therapy with \textcolor{red}{\textbf{\textless e1\textgreater steriods\textless /e1\textgreater}}, cytoxan and plasmapheresis. \end{minipage} & \begin{minipage}{6cm} Drug ($e_1$) as a part of a group of drugs recommended for $e_2$ even though outcome not explicitly stated \end{minipage} & Hinder($e_1,e_2$) \\
%     \midrule
%          \rownumber & \begin{minipage}{6cm} The \textcolor{red}{\textbf{\textless e1\textgreater back pain\textless /e1\textgreater}} was unchanged from his usual back pain, secondary to his ALL, and was not relieved by \textcolor{blue}{\textbf{\textless e2\textgreater morphine\textless /e2\textgreater}} or methadone. \end{minipage} & \begin{minipage}{6cm} Explicitly stated that the condition ($e_1$) didn't improve with the drug ($e_2$) \end{minipage} & Other \\
%     \midrule
%          \rownumber & \begin{minipage}{6cm} altered mental status was secondary to \textcolor{blue}{\textbf{\textless e2\textgreater narcotics\textless /e2\textgreater}} \textcolor{red}{\textbf{\textless e1\textgreater withdrawal\textless /e1\textgreater}}. \end{minipage} & \begin{minipage}{6cm} Phrasal entity e.g. narcotics withdrawal, lithium toxicity, benzodiazepine withdrawal, etc. decomposed into individual components as separate entities, hence non-causal. \end{minipage} & Other \\
%     \midrule
%          \rownumber & \begin{minipage}{6cm} Thus, it was believed that the pt's.\textcolor{red}{\textbf{\textless e1\textgreater altered mental status\textless /e1\textgreater}} was secondary to \textcolor{blue}{\textbf{\textless e2\textgreater narcotics\textless /e2\textgreater}} withdrawal. \end{minipage} & \begin{minipage}{6cm} Referring to incomplete span of driving entity i.e. just $e_2$ instead of $e_2$'s withdrawal that led to $e_1$  \end{minipage} & Other \\
% \end{longtable}
% \end{center}
